# Supplementary material for: Efficiently Learning Small Policies for Locomotion and Manipulation
Source: arXiv:2210.00140 source file (2022-09-30)
Supplement: Supplementary file 1 [file 9_Appendix.tex]

\section*{APPENDIX}
\label{sec:app}
\subsection{SAC Implementation details for locomotion tasks}
The same parameters were used for all locomotion tasks:\\
Number of steps trained: 3000001,
Discount Factor gamma: 0.99,
Polyak averaging tau: 0.005,
Learning rate: 0.0003, 
Entropy regularizing coefficient alpha: 0.2, 
automatic entropy tuning: false, 
batch size: 256, 
Steps to sample average actions before training: 10000, 
target update interval: 1, 
replay size: 1000000;\\
For Baseline, hidden size: 256;\\ 
For HyperPolicy, meta batch size: 8,
updates per step: 8, 
steps per arc: 100.

\subsection{DDPG-HER Implementation details for manipulation tasks}
